# Supplementary material for: Decagonal Sn clathrate on $d$-Al-Ni-Co
Source: arXiv:2212.09540 source file (2022-12-19)
Supplement: Supplementary file 1 [file Sn_AlNiCo_Supplement_prb_R2_nomarkup.pdf]

Supplementary material to the manuscript entitled:

**Decagonal Sn clathrate on *d*-Al-Ni-Co**

Vipin Kumar Singh[1], Eva Pospisilova[2], Marek Mihalkovič[2†], Marian Krajčí[2*], Pramod Bhakuni[1], Shuvam Sarkar[1], Katariina Pussi[3], D. L. Schlagel[4], T. A. Lograsso[4], Paul C. Canfield[4,5], Sudipta Roy Barman[1#]

[1]UGC-DAE Consortium for Scientific Research, Khandwa Road, Indore - 452001, Madhya Pradesh, India

[2]Institute of Physics, Slovak Academy of Sciences, Dúbravská cesta 9, SK-84511 Bratislava, Slovak Republic

[3]LUT School of Engineering Science, P.O. Box 20, FIN-53851 Lappeenranta, Finland

[4]Ames Laboratory, Iowa State University, Ames, Iowa 50011, USA

[5]Department of Physics and Astronomy, Iowa State University, Ames Iowa 50011, USA

The supplementary material contains Figures S1-S9, Tables SI-III, a note entitled "Bulk Al-Ni-Co-$R_2T_4$ approximant structure from atomistic simulation", 3 VASP CONTCAR files, and 7 video files showing LEED patterns with increasing beam energy ($E_p$), as indicated in the top left corner for each pattern appearing in the videos. The mp4 video files named by the Sn film thickness as "monolayer", "0.9nm", and "10nm" represent the 1 ML, 0.9 nm, and 10 nm Sn films on *d*-Al-Ni-Co. The video files for in-between depositions are named by the deposition time ($t_d$) as "6min", "12min", "17min", and "27min" for 6, 12, 17, and 27 minute depositions, respectively. The video and the CONTCAR files are uploaded separately.

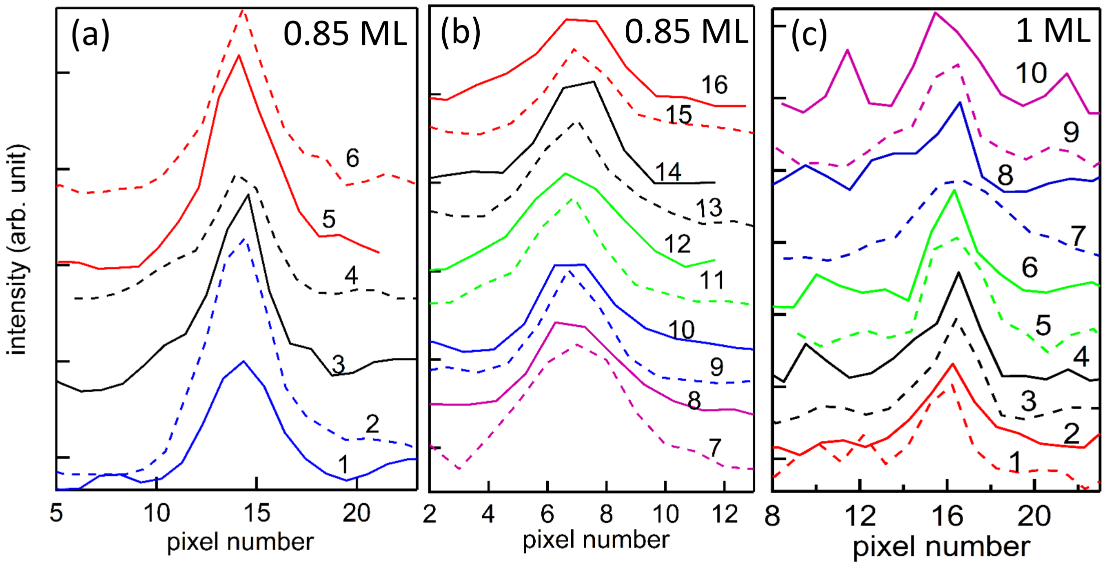


FIG. S 1. The intensity profiles of FFT spots along tangential lines through the spots for 0.85 ML (a) 1-6, (b) 7-16, and for 1 ML (d) 1-10, respectively.

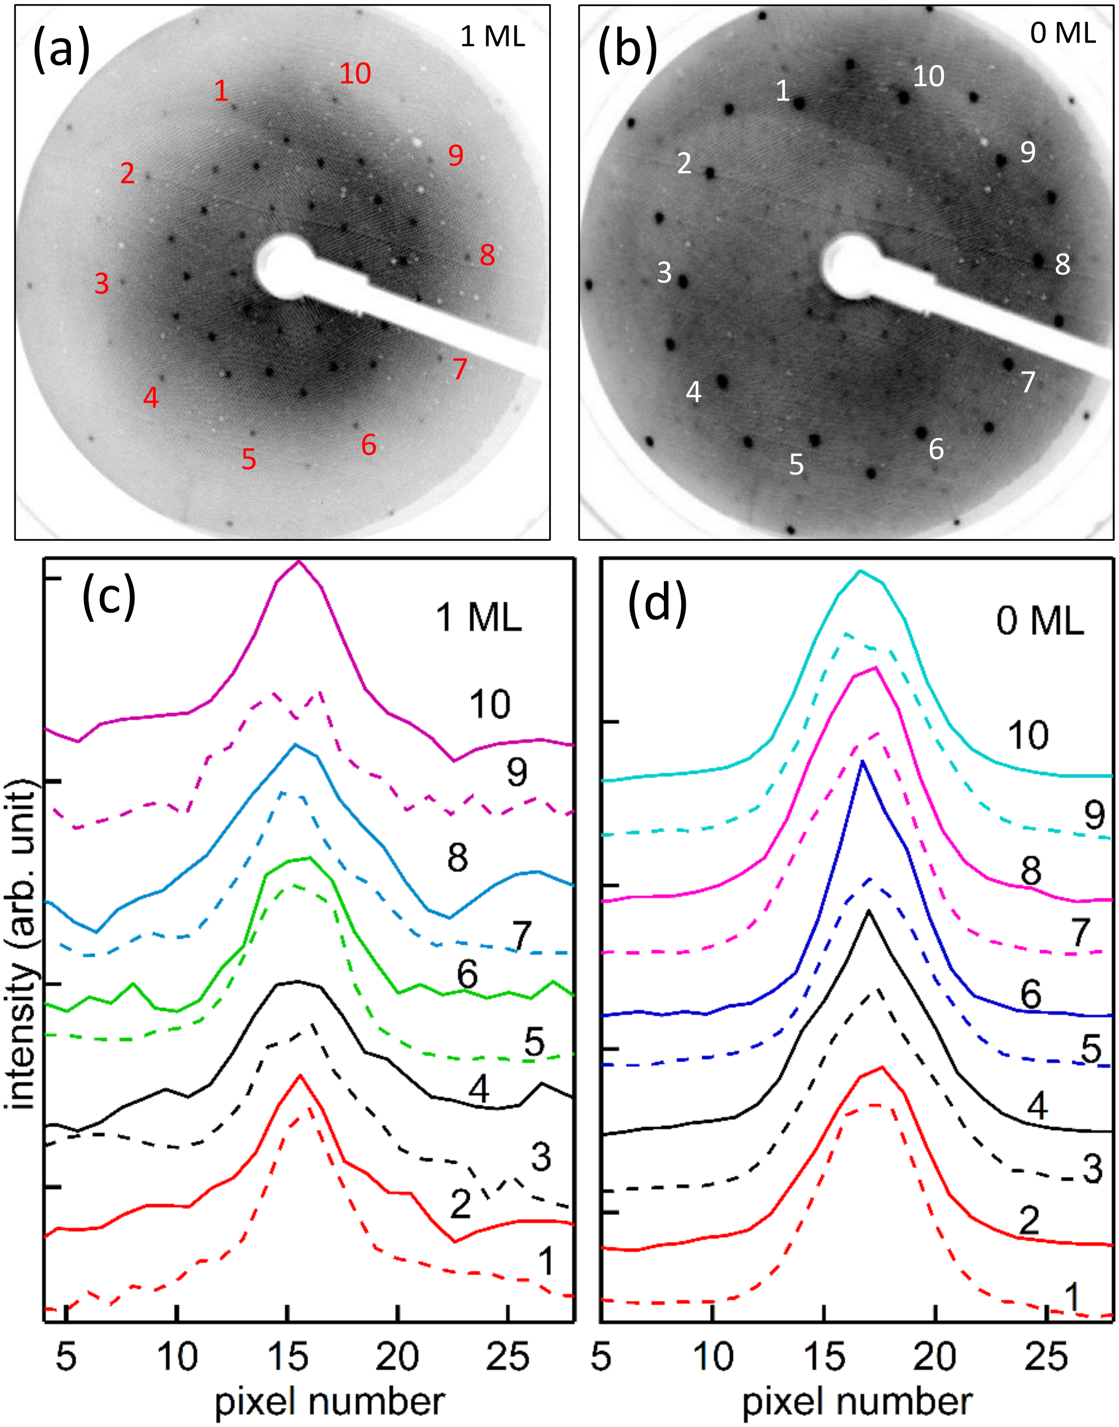


FIG. S 2. The LEED pattern of (a) 1 ML Sn/*d*-Al-Ni-Co deposited at 165±10 K (LT) is compared with (b) the substrate *d*-Al-Ni-Co, both recorded with beam energy $E_p$= 55 eV. The spots are numbered for the two outer sets. The intensity profiles along tangential lines through the LEED spots of 1-10 for (c) 1ML and (d) 0 ML, respectively.

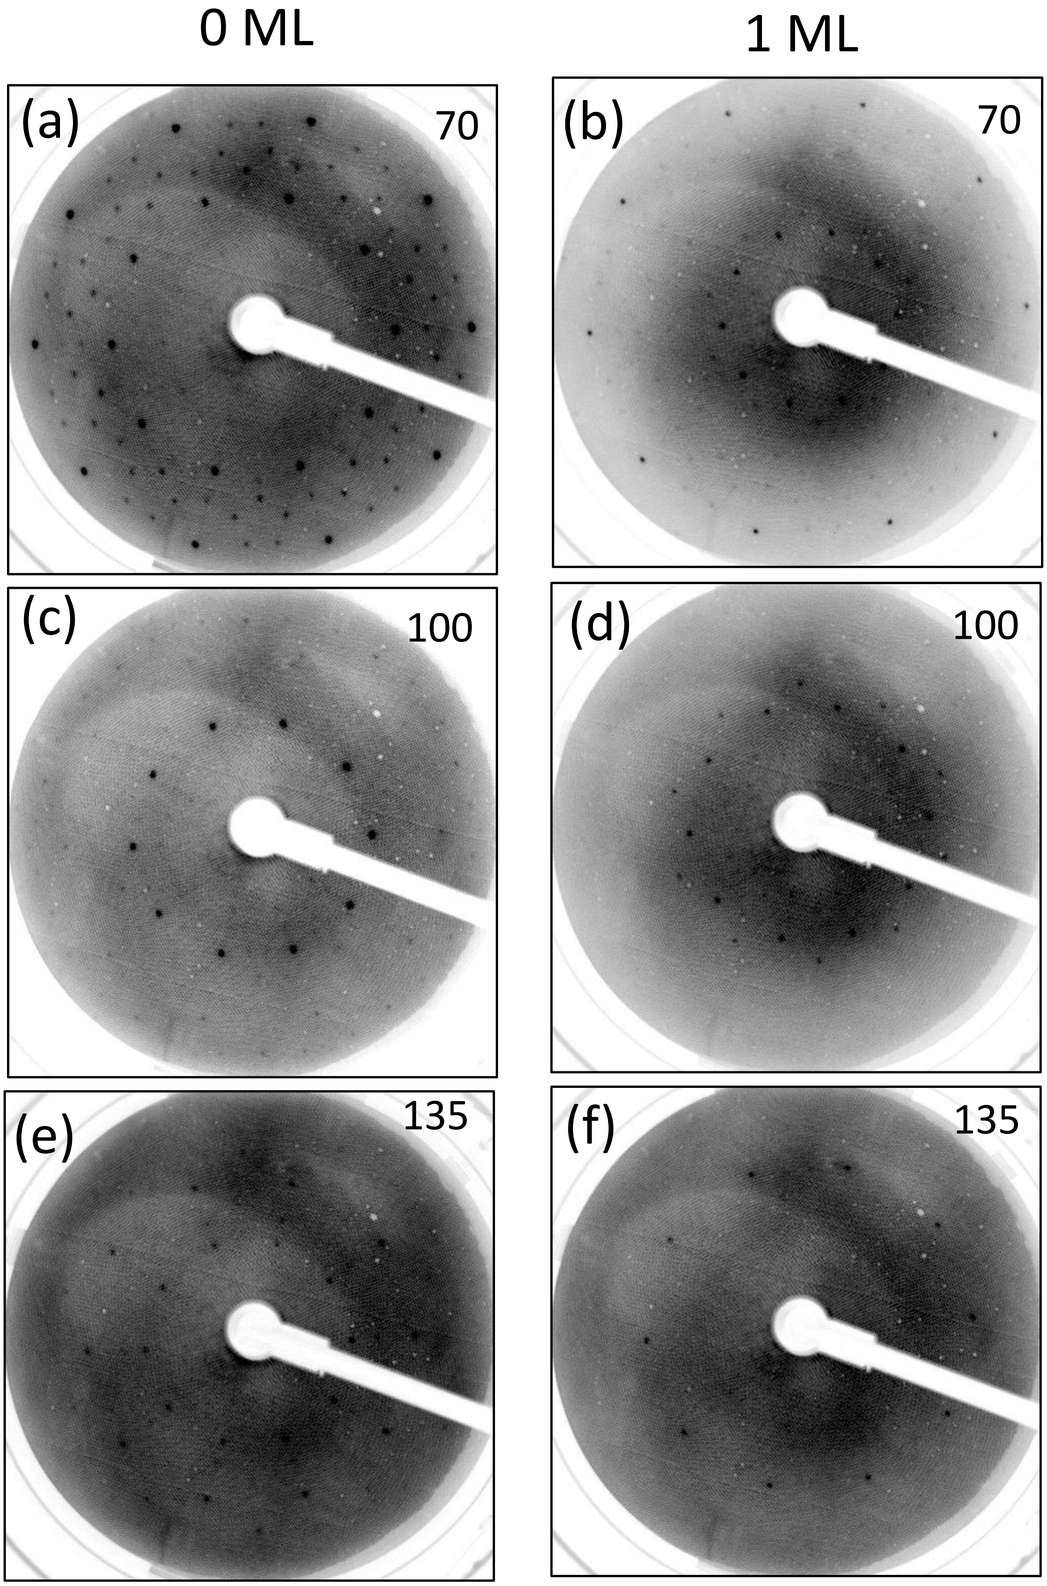


FIG. S 3. LEED patterns of (a,c,e) $d$-Al-Ni-Co and (b,d,f) 1 ML Sn/$d$-Al-Ni-Co for different beam energies ($E_p$), shown at the top right corners in eV.

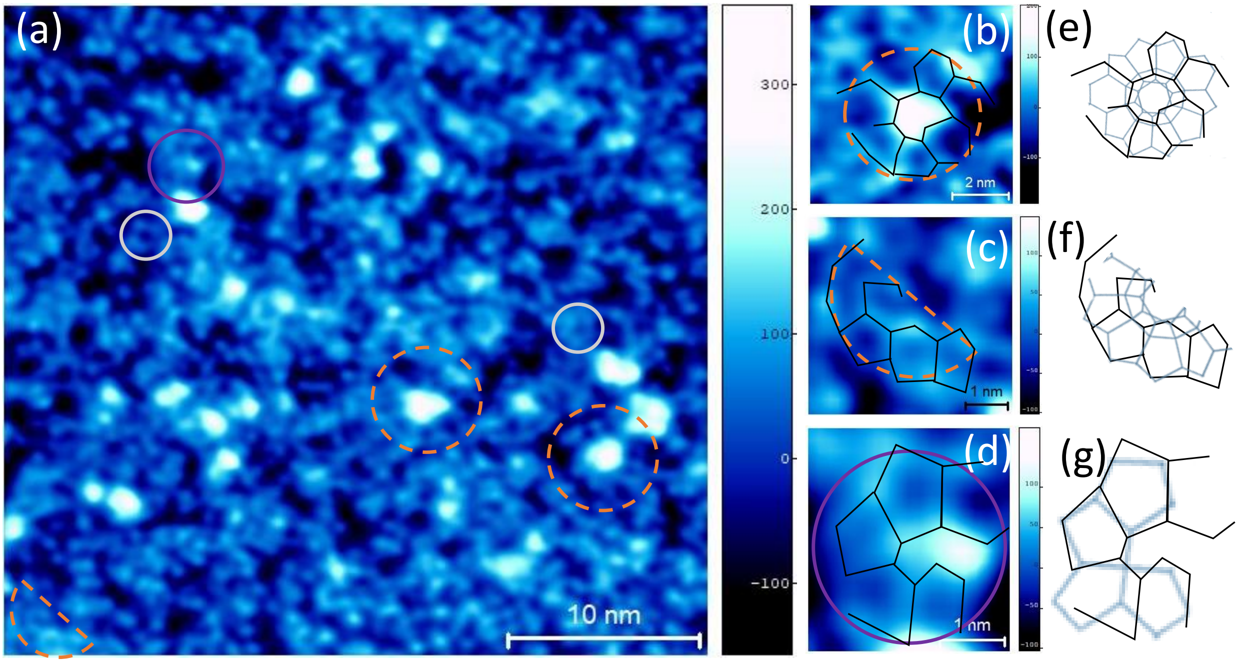


FIG. S 4. (a) STM topography image ($I_T$= 1.3 nA, $U_T$= 1.2 V) of 1 ML Sn/d-Al-Ni-Co deposited at 165±10K (LT) with the motifs highlighted. Some of these e.g. (b) wheel (dashed orange circle), (c) crown (dashed orange half-circle), and (d) polygon assembly (violet circle) are zoomed, traced (black lines) and compared in panels **e, f, g**, respectively with the energy-optimized relaxed surface of the $R_2T_4$ clathrate approximant (light blue lines) after $\tau^2$ inflation.

TABLE. S I. Ratio of the radii of different sets of 10f diffraction spots (as numbered #2- #6 ) to the radius of the innermost set of spots (set #1) for one monolayer Sn LEED pattern shown in Fig. 2(a).

| Pair of diffraction spots | Ratio from pattern | Ratio in terms of $\tau$ and $\chi$ |
|---|---|---|
| 1, 2 | 1.67 | $\tau$ (=1.618) |
| 1, 3 | 1.95 | $\tau\chi$ (=1.90) |
| 1, 4 | 2.66 | $\tau^2$ (=2.617) |
| 1, 5 | 3.08 | $\tau^2\chi$ (=3.062) |
| 1, 6 | 4.1 | $\tau^3$ (=4.235) |

TABLE. S II. Ratio of the radii of different sets of 10f diffraction spots (as numbered #2- #6 ) to the radius of the innermost set of spots (set #1) for the 0.9 nm Sn thin film shown in Fig. 3(a).

| Pair of diffraction spots | Ratio from pattern | Ratio in terms of $\tau$ and $\chi$ |
|---|---|---|
| 1, 2 | 1.67 | $\tau$ (=1.618) |
| 1, 3 | 2.0 | $\tau\chi$ (=1.90) |
| 1, 4 | 2.68 | $\tau^2$ (=2.617) |
| 1, 5 | 3.15 | $\tau^2\chi$ (=3.062) |
| 1, 6 | 4.17 | $\tau^3$ (=4.235) |

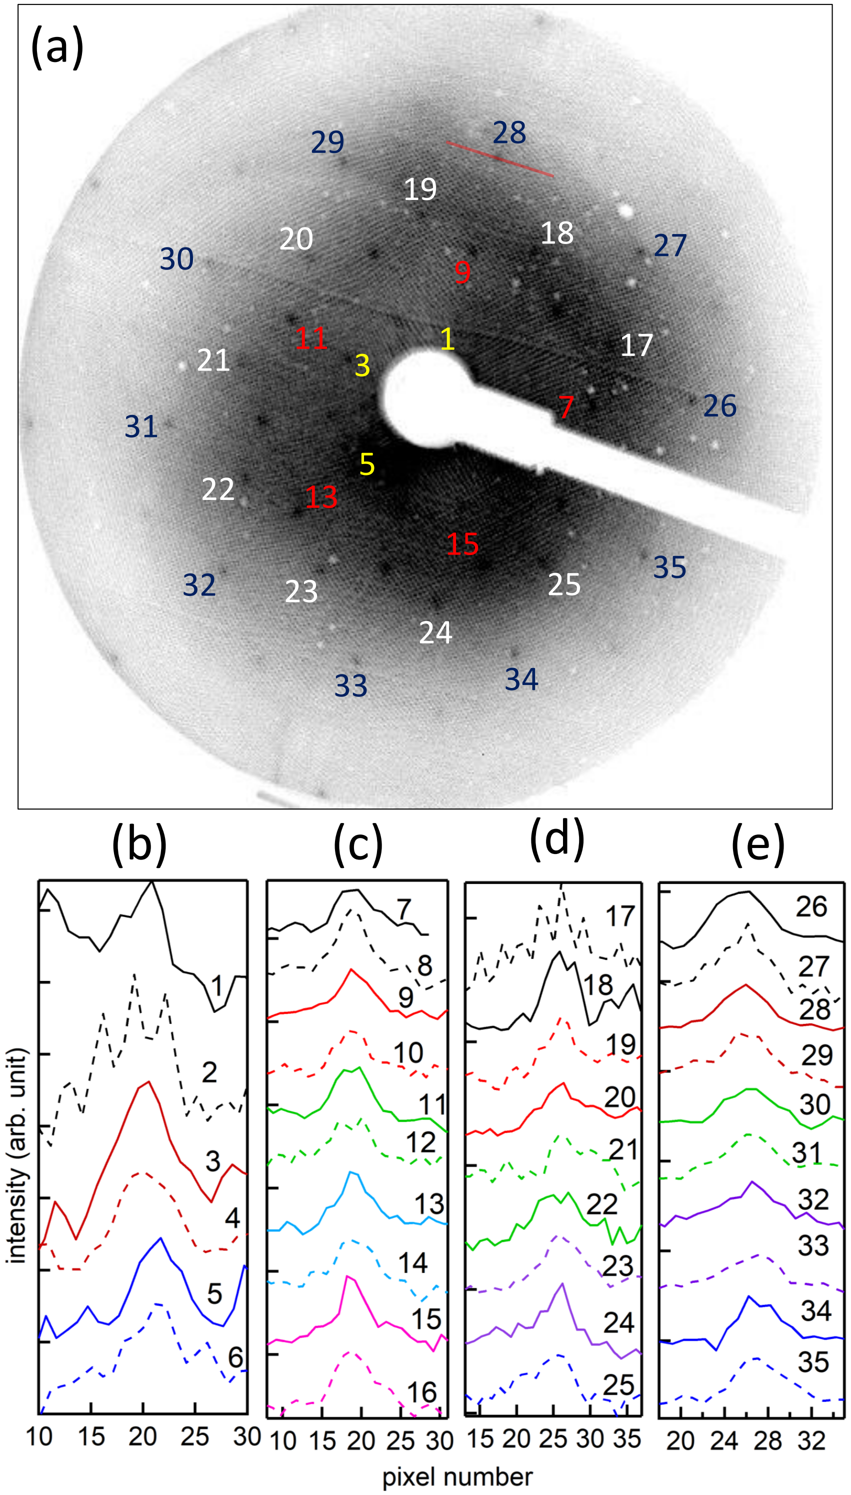


FIG. S 5. (a) LEED pattern (in inverted gray scale with Ep= 55 eV) of a 0.9 nm Sn thin film deposited at LT on *d*-Al-Ni-Co. The intensity profiles along tangential lines (*e.g.* along the red line in panel **a** for spot 28) through the spots (b) 1-6, (c) 7-16, (d) 17-25, and (e) 26-35, respectively for Sn film of intermediate thickness.

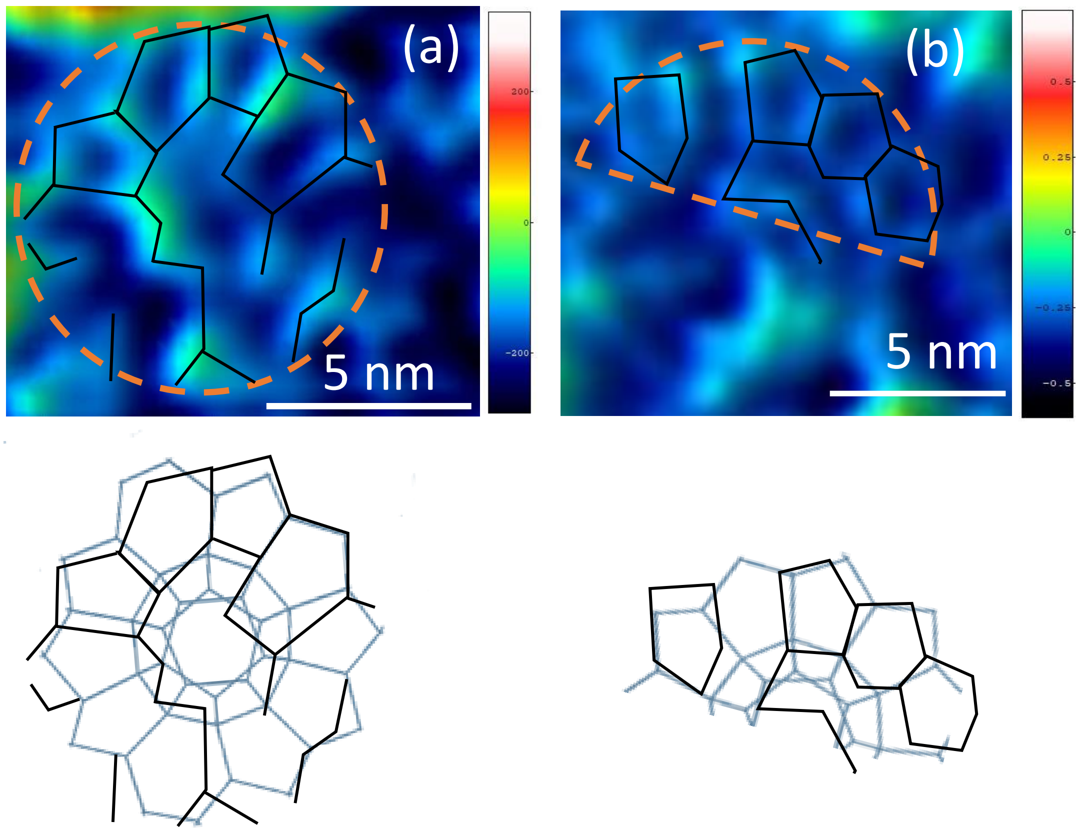


FIG. S 6. (a) The crown (dashed orange half-circle) motif and (b) the wheel (dashed orange circle) for the 0.9 nm Sn thin film are traced by black lines and compared below each image with the energy-optimized relaxed surface of the $R_2T_4$ clathrate approximant (light blue lines) after $\tau^3\chi$ inflation.

## Note: Bulk Al-Ni-Co-$R_2T_4$ approximant structure from atomistic simulation

Combining replica exchange simulation with fitted Al-Ni-Co Empirical Oscillating Pair Potentials (EOPP) [1] lead straightforwardly to realistic Al-Ni-Co structure that was unstable just by 14.6 meV/atom against decomposition into three competing crystals: $Al_3Ni_2$, $Al_9Co_2$ and $Al_3Co$ in final DFT evaluation of the total energies. The EOPP have been fitted to a "minimalistic" database containing DFT data (force components for every atom and total energy) for 6 samples : two relaxed structures (W–phase and a Ni–rich Al-Ni-Co approximant) and four snapshots from MD simulations: pure Al (4×4×4 supercell) at 600 K, two liquid samples at Co–rich and Ni–rich at 1500 K, and one under-cooled liquid sample (200 atoms each). The fit to EOPP analytical form:

$$V(r) = \frac{C1}{r^{\eta_1}} + \frac{C2}{r^{\eta_2}} \cos(k_* r + \phi_*) \quad (1)$$

converged to an excellent r.m.s. of 0.14 eV/Å$^2$ for 3621 force components and r.m.s. of 4.9

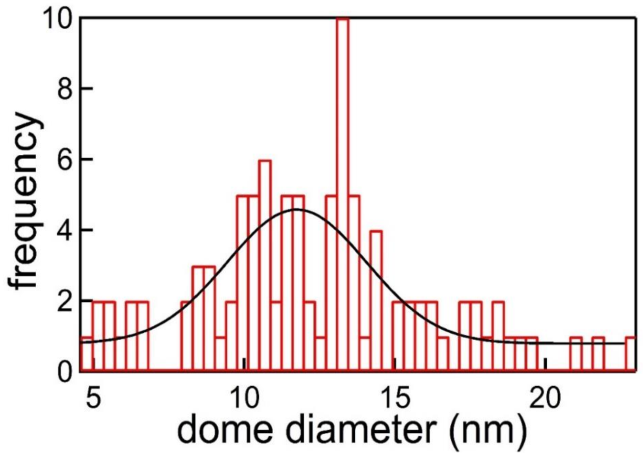


FIG. S 7. A distribution of the diameter of the domes fitted with a Gaussian curve (black line) for thick Sn film.

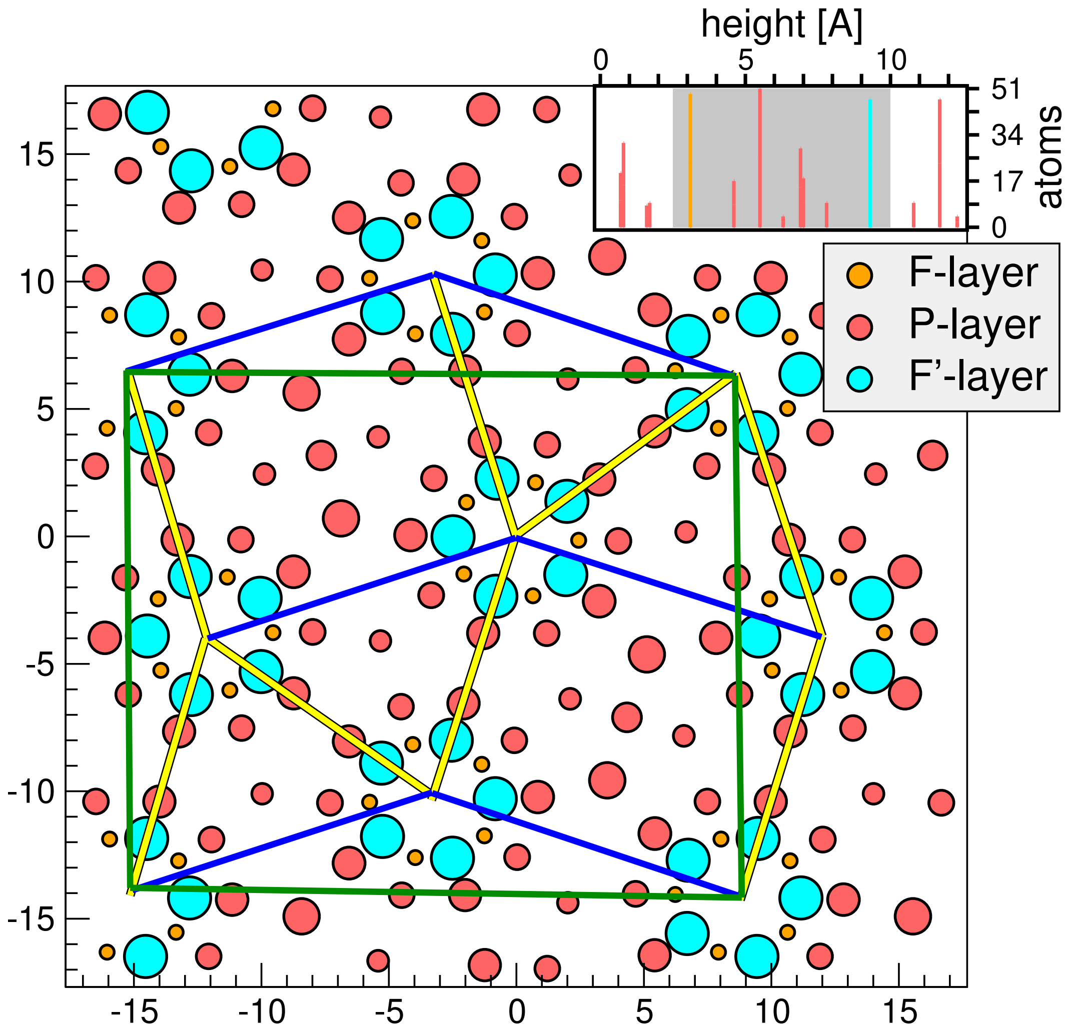


FIG. S 8. The bulk structure of the $R_2T_4$ approximant of the Sn clathrate with *Pbam* (#55) space group.

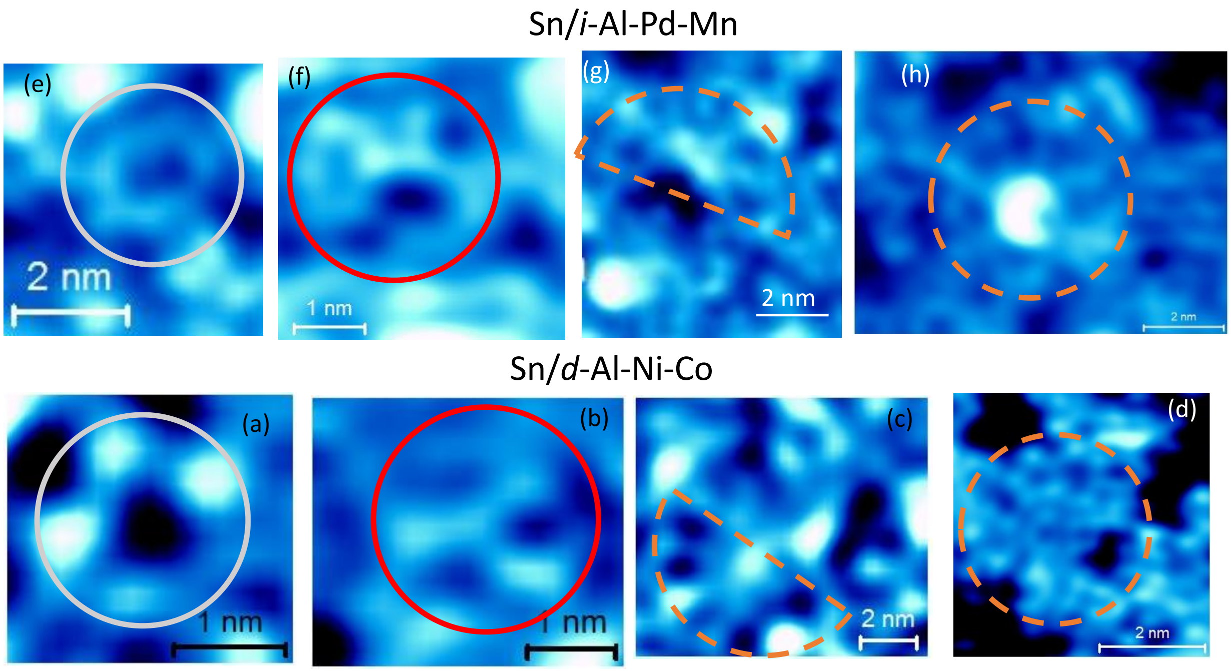


FIG. S 9. The motifs such as (a) pentagon (b) triplet, (c) crown and (d) wheel of the Sn monolayer on *i*-Al-Pd-Mn. These are compared with the motifs of Sn monolayer on *d*-Al-Ni-Co in panels **e, f, g, h**, respectively; these images are same as Figs. 16(a, b, d, e) but without the tracing.

meV/atom for formation enthalpies against tie–plane FCC-Al–AlCo.cP2–AlNi.cP2. The resulting fit parameters are in the Table SIII. The replica–exchange simulation started with $Al_{190}Co_{47}Ni_{27}$ composition in the $R_2T_4$ orthorhombic periodic cell with lattice parameters $a$= 1.983 nm, $b$= 2.339 nm and $c$= 0.815 nm. Tempering simulation proceeded at six temperatures in the range 600 K–967 K, repeating iteratively 30000 times elementary update-cycle, consisting of 200 MD steps followed by 30 chemistry swap attempts per pair of atoms. At the end of the simulation, we picked lowest-energy sample from the database of stored 600 K samples, and performed full structure/cell DFT optimization, leading to the cell parameters $a$= 1.980 nm, $b$= 2.332 nm and $c$= 0.812 nm.

Our final structure had 264 atoms/cell and a composition of $Al_{190}Co_{47}Ni_{27}$. To evaluate goodness of the structure model we computed its total DFT energy and determined $\Delta E$ from the tie-plane of the competing crystal phases ($Al_3Ni_2$–$Al_9Co_2$–$Al_3Co$) to be +14.6 meV/atom, as compared to +11.0 meV/atom for the experimentally refined to the cell doubling of the W–phase offers finite but rather small energy advantage of ∼+4 meV/atom over the fundamental-cell model developed here.

TABLE. S III. EOPP parameters for Al-rich Al-Ni-Co system between Sn-clathrate film and Al-Ni-Co substrate.

| | C1 | $\eta_1$ | C2 | $\eta_2$ | $K_*$ | $\phi_*$ |
|---|---|---|---|---|---|---|
| Al-Al | 884.25 | 8.570 | -1.576 | 3.760 | 3.571 | 2.740 |
| Al-Co | 522.37 | 9.702 | 5.627 | 3.685 | 3.064 | 1.851 |
| Al-Ni | 333.41 | 8.730 | 3.557 | 3.474 | 3.141 | 1.759 |
| Co-Co | 160.16 | 6.236 | -1.205 | 2.356 | -2.980 | 0.450 |
| Co-Ni | 142.67 | 6.135 | -2.572 | 2.863 | -2.907 | 0.228 |
| Ni-Ni | 265.39 | 7.399 | -0.977 | 2.445 | -2.978 | 0.479 |

Fig. 14(a) displays $R_2T_4$-Al-Ni-Co bilayer at the $B$–type surface analogical to its W-phase counterpart in Fig. 12(b): the so called pentagonal-bipyramid column – the fundamental motif of the $Al_{13}Co_4$ structure – around the rightmost solid red pentagon in the Fig. 12(b) exactly corresponds to the column marked by blue circle in Fig. 14(a). The red and green circles mark in turn the columns analogical to the dashed-red pentagon in Fig. 12(b), while the red/green assignments only differ by Co/Ni assignment. Finally, the black-circle marked column also has exact analogue in W–phase – in Fig. 12(b) it is linked by blue linkage to the rightmost solid–red-pentagon column. We conclude that the crucial feature of the cell-doubling symmetry-breaking in W-structure is 4 Å vertical shift of the pentagonal–bipyramid column between adjacent cells, bringing it few meV/atom energetic advantage over the current fundamental cell structure.

[1] M. Mihalkovič, C. L. Henley, Phys. Rev. B **85**, 092102 (2012).

[2] V. K. Singh, M. Mihalkovič, M. Krajčí, S. Sarkar, P. Sadhukhan, M. Maniraj, A. Rai, K. Pussi, D. L. Schlagel, T. A. Lograsso, A. K. Shukla, and S. R. Barman, Phys. Rev. Res. **2**, 013023 (2020).
